# Supplementary material for: DarkShake-DVS: Event-based Human Action Recognition under Low-light andShaking Camera Conditions
Source: arXiv:2605.20680 source file (2026-05-20)
Supplement: Supplementary file 1 [file 12_appendix.tex]

\section{Appendix Section}
\label{sec:appendix_section}
Supplementary material goes here.
