# Supplementary material for: DarkShake-DVS: Event-based Human Action Recognition under Low-light andShaking Camera Conditions
Source: arXiv:2605.20680 source file (2026-05-20)
Supplement: Supplementary file 2 [file X_suppl.tex]

\clearpage
\setcounter{page}{1}
\maketitlesupplementary
\begin{table*}[t]
\centering
% 必须使用极小字体，否则10列放不下
\scriptsize 
%\footnotesize % 如果你的类别名都很短（1个单词），可以尝试这个稍大一点的字体

% 去除额外间距，保持紧凑

% 定义列格式：5组 (序号居中 + 类别自动宽)
% c X c X c X c X c X
\begin{tabularx}{\textwidth}{c X c X c X c X c X}
\toprule
\textbf{No.} & \textbf{Class} & \textbf{No.} & \textbf{Class} & \textbf{No.} & \textbf{Class} & \textbf{No.} & \textbf{Class} & \textbf{No.} & \textbf{Class} \\
\midrule
1  & Holding head  & 2  & Holding stomach    & 3  & Waving  & 4  & Standing up   & 5  & Pulling door    \\
6  & Drinking    & 7  & Walking stooped   & 8  & Walking holding wall   & 9  & Sitting down   & 10 & Squatting   \\
11  & Crossing arms    & 12  & Sitting down   & 13  & Bowing holding wall   & 14  & Punching   & 15 & Running   \\
16  & Holding back of head    & 17  & Walking down stairs   & 18  & Reading book   & 19  & Picking up chair   & 20 & Waving both hands   \\

21  & Sweeping    & 22  & Dancing   & 23  & Cutting vegetables   & 24 & Stir-frying   & 25 & Brushing hair   \\
26  & Wiping face    & 27  & Knitting sweater   & 28  & Washing face   & 29 & Washing clothes   & 30 & Beating quilt   \\
31  & Clapping    & 32  & Putting hands on hips   & 33  & Shaking hands   & 34 & Saluting   & 35 & Sitting down (paired)   \\
36  &  Fist bumping    & 37  & Hitting   & 38  & Performing CPR   & 39 & Giving chair and sitting down   & 40 & Playing tug of war   \\
41  & Reading (paired)    & 42  & High fiving   & 43  & Hugging   & 44 & Rock-paper-scissors   & 45 & Holding umbrella   \\
46  & Typing    & 47  & Playing football   & 48  & Walking arm on shoulder   & 49 & Putting on hat   & 50 & Kicking   \\
51  & Following    & 52  & Patting shoulder   & 53  & Arm wrestling   & 54 & Cutting hair   & 55 & Playing handball   \\
56  & Swinging jump rope    & 57  & Dancing in pairs   & 58  & Hammering nail   & 59 & Repairing bicycle   & 60 & Doing burpees (paired)   \\
61 & Latin dancing  & 62 & Shaking out clothes  &    &            &    &            &    &            \\
\bottomrule
\end{tabularx}
\caption{\textit{Full list of the 62 action categories in the DarkShake-DVS dataset.}}
\label{table:full_action_list}
\vspace{-5mm}
\end{table*}

% \section{Abstract}
% \label{sec:abstract}

% In this supplementary material, we provide additional details to support the contributions of the main paper. First, in Section 2, we elaborate on the DarkShake-DVS dataset, presenting visualizations of the recording scenes and viewpoints, the complete list of action categories, and a quantitative assessment of the illumination conditions. We also discuss the rationale behind the Event-IMU complementarity and outline the ethical considerations for data collection. Next, in Section 3, we supply the specific parameter settings for the Adaptive Motion Compensation module and the Informative Group Sampling (IGS) strategy. Finally, we present the detailed pseudocode and implementation logic for the Adaptive IMU Grouping and Scaling algorithm.

\section{More Details of Dataset}

\begin{figure}
    \centering
  \includegraphics[scale=0.7]{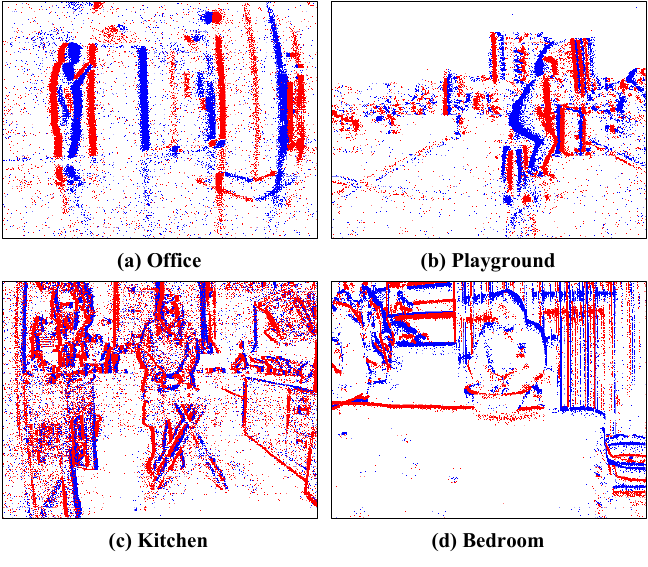}
  \captionsetup{skip=-0.1mm}
    \caption{ 
    \textit{Visualization of representative recording scenes, including offices, playgrounds, kitchens, and bedrooms.}}
    \label{fig:scenes}
\vspace{-5mm}
\end{figure}

\textbf{Visualization of Categories, Scenes, and Viewpoints.} To provide a comprehensive overview of the DarkShake-DVS dataset and substantiate the descriptions in the main paper, we present detailed visualizations of the data distribution. First, the complete list of all action categories is enumerated in Tab.~\ref{table:full_action_list}. To demonstrate the environmental diversity mentioned in the main text, Fig.~\ref{fig:scenes} displays representative samples from various recording environments, including offices, playgrounds, kitchens, and bedrooms, containing both static and dynamic background elements. Furthermore, to illustrate the extensive geometric coverage, Fig.~\ref{fig:viewpoints} showcases samples captured from multiple distinct viewpoints. As described in the collection process, these include the front, back, left, right, and four diagonal directions, ensuring the dataset covers a full spectrum of observation angles under realistic 6-DoF camera motion.

\begin{algorithm}[t]\caption{Adaptive IMU Grouping and Scaling Algorithm}\label{alg:imu_grouping}\small\textbf{Input:} IMU angular velocity sequence $\boldsymbol{\omega} = \{\omega_1, \dots, \omega_T\}$, IMU timestamps $\mathbf{t}$, Thresholds $T_{\text{stable}}$, $N_{\min}$, $N_{\max}$. \\textbf{Output:} Set of compensation groups $\mathcal{G} = \{G_1, \dots, G_M\}$, Scaling factors $\boldsymbol{\gamma}$.\begin{algorithmic}[1]\STATE \textbf{Stage 1: Initial Segmentation}\STATE Initialize $\mathcal{G}_{\text{raw}} \leftarrow \emptyset$\FOR{each timestamp $t$}\IF{$|\omega_t| \le T_{\text{stable}}$}\STATE Mark $\omega_t$ as \textit{Stable}; group consecutive stable points into $\mathcal{G}_{\text{raw}}$.\ELSE\STATE Mark $\omega_t$ as \textit{Active}; group consecutive active points into $\mathcal{G}_{\text{raw}}$.\ENDIF\ENDFOR\STATE \textbf{Stage 2: Hierarchical Refinement (for Active Groups)}\STATE Initialize $\mathcal{G}_{\text{refined}} \leftarrow \emptyset$\FOR{each group $G \in \mathcal{G}_{\text{raw}}$ where type is \textit{Active}}\STATE \COMMENT{Step 2.1: Split by Polarity}\STATE Split $G$ into sub-segments $\{S_1, \dots\}$ where $\text{sgn}(\omega)$ is constant.\FOR{each sub-segment $S \in \{S_1, \dots\}$}
    \STATE \COMMENT{Step 2.2: Split by Extrema (Peak)}
    \STATE Find peak index $k = \arg\max_{t \in S} |\omega_t|$.
    \STATE Split $S$ into $S_{\text{acc}} = S[0:k]$ and $S_{\text{dec}} = S[k+1:end]$.
    
    \FOR{each phase $P \in \{S_{\text{acc}}, S_{\text{dec}}\}$}
        \STATE \COMMENT{Step 2.3: Split by Cumulative Energy}
        \STATE Calculate total energy $E = \sum |\omega_t|$.
        \STATE Find split point $j$ where $\sum_{t=0}^j |\omega_t| \approx E / 2$.
        \STATE Split $P$ into $P_{\text{early}}, P_{\text{late}}$ at index $j$.
        \STATE Add $P_{\text{early}}, P_{\text{late}}$ to $\mathcal{G}_{\text{refined}}$.
    \ENDFOR
\ENDFOR
\ENDFOR\STATE Add \textit{Stable} groups from $\mathcal{G}_{\text{raw}}$ directly to $\mathcal{G}_{\text{refined}}$.\STATE \textbf{Stage 3: Temporal Regularization \& Scaling}\STATE Sort $\mathcal{G}_{\text{refined}}$ by time.\STATE \textbf{Merge:} Combine adjacent groups if length $< N_{\min}$.\STATE \textbf{Split:} Recursively divide groups if length $> N_{\max}$.\STATE \textbf{Calculate:} For each final group $G_k$, compute $\gamma_k$:\STATE $\gamma_k \leftarrow \gamma_{\min} + \frac{\gamma_{\max} - \gamma_{\min}}{a \cdot |G_k| + b}$\RETURN Final Groups $\mathcal{G}$, Scaling Factors $\boldsymbol{\gamma}$\end{algorithmic}\end{algorithm}

\noindent\textbf{Illumination Condition Details.} To quantitatively assess the low-light conditions of our DarkShake-DVS dataset, we measured the ambient illumination using a DLX-SL138 digital lux meter. The measurements confirmed an average illuminance of 1-3 Lux across our recording scenes. This illuminance level verifies that the dataset was captured under significant low-light conditions. For traditional frame-based cameras, such low illumination would drastically reduce the signal-to-noise ratio (SNR) and lead to severe motion blur \cite{wang2024hardvs, liu2022video, zhouspikformer, li2024videomamba}, especially when combined with the 6-DoF motion central to our work \cite{hutagalung2023effectiveness}. However, as discussed in the main paper, event cameras possess high dynamic range \cite{10.1007/978-3-031-72775-7_17} and high low-light sensitivity \cite{Pan_2019_CVPR} . They operate by capturing microsecond-level relative changes in brightness rather than absolute illumination. Therefore, while an environment of 1-3 Lux is challenging for traditional cameras, it represents an ideal regime that is effectively captured by event cameras, highlighting their advantages in low-noise signal acquisition. This makes our dataset a robust and realistic benchmark for evaluating the performance of HAR methods in challenging real-world low-light scenarios.

\begin{figure}
    \centering
  \includegraphics[scale=0.7]{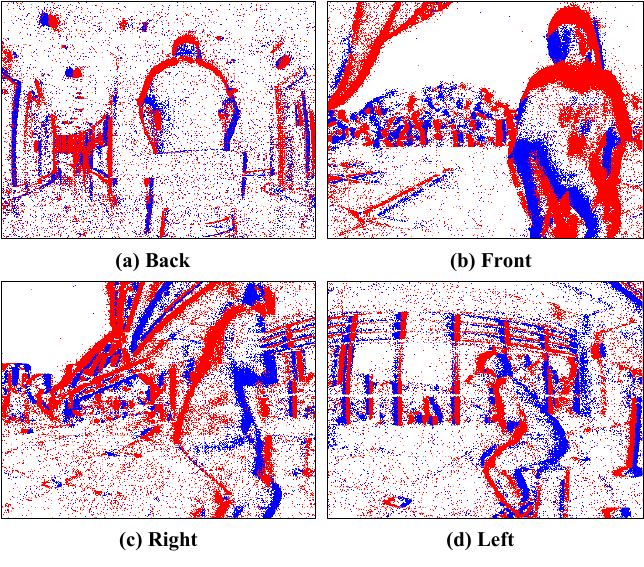}
  \captionsetup{skip=-0.1mm}
    \caption{ 
    \textit{Visualization of samples from diverse viewpoints, including front, back, side, and diagonal angles. }}
    \label{fig:viewpoints}
\vspace{-5mm}
\end{figure}

\noindent\textbf{Event–IMU Complementarity} In our work, pairing the event camera with an IMU is crucial for addressing the challenge of 6-DoF motion. Unconstrained camera shake generates a high volume of background events, which contaminate the foreground events caused by the human action, severely interfering with recognition. The unique advantage of the IMU is its ability to independently and accurately measure the camera's own motion , such as angular velocity and acceleration, with performance that is completely unaffected by lighting conditions. In our low-light dataset, where visual-only motion estimation algorithms would fail, the IMU consistently provides reliable motion data. Therefore, we can leverage the precise ego-motion information from the IMU to compensate and stabilize the event stream, thereby isolating the true human action. This tight coupling of Event-IMU data is an industry and academic consensus; many advanced commercial event cameras, such as the DVXplorer natively integrate an IMU, confirming the validity of our method and dataset design.

\noindent\textbf{Data Collection and Ethics.} Taking into account the sensitive nature of our dataset, all data involving human participants were collected in accordance with informed consent procedures. Participants were fully informed about the purpose of the study, the nature of their participation, potential risks, benefits, and their right to withdraw from the study at any time without suffering any adverse consequences.

\section{Parameter Settings}
\textbf{Adaptive Motion Compensation.} In the proposed IMU-temporal-aware dynamic scaling mechanism, the scaling factor $\gamma_{\text{group}}$ is adjusted based on the IMU sample density $N_{\text{imu}}$. The bounds for the scaling factor are set to $\gamma_{\min} = $ 2 and $\gamma_{\max} = $ 5. The tuning coefficients in the denominator, which control the sensitivity of the scaling to the sample count, are set to $a = $ 0.15 and $b = $ 3, respectively. These values were empirically determined to balance motion suppression and feature preservation.IGS Algorithm. In the Informative Group Sampling (IGS) strategy, the comprehensive score $S_{\text{comb}}(i)$ is a weighted sum of four metrics: relevance, quality, uniformity, and diversity. We assign the weights as follows: the relevance weight $w_{\text{rel}} = $ 0.1, the quality weight $w_{\text{q}} = $ 0.1, the uniformity weight $w_{\text{u}} = $ 0.6, and the diversity weight $w_{\text{d}} = $ 0.1. The higher weights on uniformity are higher, indicating that we prioritize semantic alignment during the frame selection process.

\noindent\textbf{Detailed Algorithm for Adaptive Motion Compensation.} To provide a comprehensive understanding of our adaptive motion compensation framework, we present the detailed algorithmic procedure for IMU data grouping and dynamic scaling factor calculation. As described in the main paper, our goal is to partition the continuous angular velocity sequence into fine-grained, motion-consistent groups. While the main text outlines the frequency-domain conceptualization, the practical implementation involves a hierarchical segmentation strategy followed by a regularization process.The specific grouping process, as outlined in Algorithm \ref{alg:imu_grouping}, consists of three primary stages. (1) Initial Segmentation: We first separate the IMU sequence into "stable" and "active" segments based on a noise threshold (set to $\pm 3$ rad/s in our experiments). Stable regions represent static or micro-motion phases, while active regions contain significant camera ego-motion. (2) Hierarchical Refinement: For active segments, we apply a three-step refinement to capture motion dynamics: Sign-based Splitting ensures each group maintains a monotonic direction; Extrema-based Splitting divides the motion into acceleration and deceleration phases by cutting at the peak angular velocity; and Energy-based Splitting further subdivides high-energy segments at the median point of their cumulative angular displacement (energy), ensuring a balanced motion distribution within groups. (3) Temporal Regularization: To satisfy the temporal constraints of the event camera, we perform a post-processing step where groups smaller than a minimum duration ($N_{min}$) are merged into adjacent groups, and groups exceeding a maximum duration ($N_{max}$) are recursively split. Finally, the dynamic scaling factor $\gamma_{\text{group}}$ is computed for each valid group to guide the event warping process.
